# Supplementary material for: Intertwined Magnetism and Superconductivity in Isolated Correlated Flat Bands
Source: arXiv:2402.09506 source file (2024-07-07)
Supplement: Supplementary file 1 [file supplementary_standalone.tex]

\documentclass[aps,prl,
twocolumn,
floatfix,longbibliography,nofootinbib,tbtags]{revtex4-1}
\usepackage[utf8]{inputenc}
\usepackage{natbib}
\usepackage{graphicx}
\usepackage{xcolor}
\usepackage{mathtools}
\usepackage{amsmath}
\usepackage[colorlinks, linkcolor=blue]{hyperref}
\hypersetup{colorlinks,allcolors=black}
\usepackage{amssymb}
\usepackage{gensymb}
\usepackage{float}
\usepackage{xr}
\externaldocument[]{main}

\newcounter{indice}

\usepackage[compat=1.1.0]{tikz-feynman}
\tikzset{
pattern size/.store in=\mcSize, 
pattern size = 5pt,
pattern thickness/.store in=\mcThickness, 
pattern thickness = 0.3pt,
pattern radius/.store in=\mcRadius, 
pattern radius = 1pt}

\usepackage{amssymb}
\newcommand{\be}{\begin{equation}}
\newcommand{\ee}{\end{equation}}
\newcommand{\beq}{\begin{eqnarray}}
\newcommand{\eeq}{\end{eqnarray}}
\newcommand{\ba}{\[\begin{aligned}}
\newcommand{\ea}{\end{aligned}\]}
\newcommand{\bal}{\begin{aligned}}
\newcommand{\eal}{\end{aligned}}

\renewcommand{\epsilon}{\varepsilon}

\def \ba{\begin{align*}}
\def \ea{\end{align*}}

\begin{document}

\bibliographystyle{apsrev4-2}
\bibliography{bib}

\end{document}
